# Supplementary material for: On the Exploration of LM-Based Soft Modular Robot Design
Source: arXiv:2411.00345 source file (2024-11-01)
Supplement: Supplementary file 1 [file appendix.tex]

% \section{Supplementary Figures}




% \begin{figure}[htbp]
%     \centering
%     \subfloat[]{%
%         \includegraphics[width=0.16\linewidth]{figures/eval-our-model/robot_plot_our-model-flat-good1.png}
%         \label{fig:ownmodel:subfig1}
%     }\hfill
%     \subfloat[]{%
%         \includegraphics[width=0.16\linewidth]{figures/eval-our-model/robot_plot_our-model-reverse-good1.png}
%         \label{fig:ownmodel:subfig3}
%     }\hfill
%     \subfloat[]{%
%         \includegraphics[width=0.16\linewidth]{figures/eval-our-model/robot_plot_our-model-downstairs-good1.png}
%         \label{fig:ownmodel:subfig5}
%     }
%     \caption{Examples of \textbf{our model} for unidirectional locomotion tasks (a),  back-and-forth locomotion tasks (b),  and descending tasks (c)}
%     \label{fig:ownmodel}
% \end{figure}

% \begin{figure}[htbp]
%     \centering
%     \subfloat[]{%
%         \includegraphics[width=0.16\linewidth]{figures/no compare/no-compare-2.png}
%         \label{fig:compare-related:subfig2}
%     }\hfill
%     \subfloat[]{%
%         \includegraphics[width=0.16\linewidth]{figures/compare-only/compareonly-1.png}
%         \label{fig:compare-related:subfig3}
%     }\hfill
%     \caption{Examples of \textbf{no-Compare} model (a) and \textbf{no-CLM} model (b)}
%     \label{fig:compare-related}
% \end{figure}

% \begin{figure}[htbp]
%     \centering
%     \subfloat[]{%
%         \includegraphics[width=0.16\linewidth]{figures/downsample/40-2.png}
%         \label{fig:downsample:subfig2}
%     }\hfill
%     \subfloat[]{%
%         \includegraphics[width=0.16\linewidth]{figures/downsample/60-2.png}
%         \label{fig:downsample:subfig4}
%     }\hfill
%     \subfloat[]{%
%         \includegraphics[width=0.16\linewidth]{figures/downsample/80-2.png}
%         \label{fig:downsample:subfig6}
%     }
%     \caption{Examples of using different size of training data: \textbf{0.4T} (a),  \textbf{0.6T} (b) ,  and \textbf{0.8T} (c)}
%     \label{fig:downsample}
% \end{figure}


% \begin{figure}[htbp]
%     \centering
%     \subfloat[]{%
%         \includegraphics[width=0.16\linewidth]{figures/12-13/12-2.png}
%         \label{fig:12_13:subfig2}
%     }\hfill
%     \subfloat[]{%
%         \includegraphics[width=0.16\linewidth]{figures/12-13/13-1.png}
%         \label{fig:12_13:subfig3}
%     }\hfill
%     \caption{Examples of \textbf{uni-downstairs}  (a) (b), and \textbf{uni-back} (c) (d)}
%     \label{fig:12_13}
% \end{figure}









% \begin{figure}[htbp]
%     \centering
%     \includegraphics[width=1\linewidth]{figures/actuation_signals-8-robots.png}
%     \caption{Control sequence for 5-module 2-leg robot locomotion.}
%     \label{fig:controlsequence_5}
% \end{figure}

% \begin{figure}[h]
%     \centering
%     \includegraphics[width=1\linewidth]{figures/actuation_signals-8-robots.png}
%     \caption{Control sequence for 5-module 'L'-shape robot locomotion.}
%     \label{fig:controlsequence_L}
% \end{figure}


% \begin{figure}[htbp]
%     \centering
%     \includegraphics[width=1\linewidth]{figures/actuation_signals-8-robots.png}
%     \caption{Control sequence for 4-module 1-chain robot locomotion.}
%     \label{fig:controlsequence_4}
% \end{figure}


% \begin{figure}[htbp]
%     \centering
%     \includegraphics[width=1\linewidth]{figures/actuation_signals-8-robots.png}
%     \caption{Control sequence for 7-module 2-leg robot locomotion.}
%     \label{fig:controlsequence_7}
% \end{figure}


% \begin{figure}[htbp]
%     \centering
%     \includegraphics[width=\linewidth]{figures/actuation_signals-8-robots.png}
%     \caption{Control sequence for 8-module 3-leg robot locomotion.}
%     \label{fig:controlsequence_8}
% \end{figure}
